# Supplementary material for: RTLRewriter: Methodologies for Large Models aided RTL Code Optimization
Source: arXiv:2409.11414 source file (2024-09-04)
Supplement: Supplementary file 1 [file appendix.tex]

\section*{Appendix}
In the appendix, we provide more details of experiments, methods and datasets.
We provide multimodal Verilog code optimization datasets, prompts details, and generation results of baselines in supplementary materials.
\section{Details of Datasets} \label{sec:data-opt}
In this paper, we propose a novel multimodal Verilog code optimization dataset. We provide more details including Verilog code instance, associated multimodalities, and optimization instructions.
\textbf{Note that none of these optimization instructions and algorithms are included in our database for RAG.}

In the realm of data-path optimization, as shown in~\Cref{table:examples}, our focus primarily lies on techniques such as  subexpression elimination \cite{cocke1970global, pasko1999new}, Constant folding~\cite{cocke1970global}, Constant propagation~\cite{wegman1991constant, metzger1993interprocedural}, Algebraic simplification~\cite{buchberger1982algebraic, carette2004understanding}, Dead code elimination \cite{knoop1994partial, gupta1997path}, and Strength reduction \cite{cooper2001operator}.
When it comes to Mux optimization, our considerations revolve around Mux reduction \cite{chen2004register, wang2023optimization}, Mux tree decomposition \cite{pivstekareduction}, and Mux tree restructuring \cite{wang2023optimization}.
In regard to memory optimization, we delve into various areas such as memory sharing \cite{laforest2010efficient, ma2020hypervisor}, memory folding, memory banking \cite{zhou2017new,lai2019remap+} and memory pipelining \cite{park2001synthesis} into consideration.
Lastly, for FSM design, we consider techniques such as state minimization \cite{kam2013synthesis}, state assignment \cite{villa2012synthesis}, and state decomposition \cite{shelar1999decomposition}.

\begin{table}[th!]
    \centering
    \caption{RTL code optimization examples}
    \resizebox{.8\linewidth}{!}
    {
        {
    \begin{tabular}{c|c|c}
    \toprule
     Class &  Strategy & Target  \\ \midrule
     Datapath        & Subexpression elimination \cite{cocke1970global, pasko1999new}& Delay, Power, Area \\
                  & Constant folding~\cite{cocke1970global} & Delay, Power, Area \\
                  & Constant propagation~\cite{wegman1991constant, metzger1993interprocedural} & Delay, Power, Area \\
                  & Copy propagation~\cite{vanbroekhoven2003advanced, metzger1993interprocedural} & Delay, Power, Area \\
                  & Algebraic simplification~\cite{buchberger1982algebraic, carette2004understanding} &  Delay, Power, Area, \\
                  & Dead code elimination \cite{knoop1994partial, gupta1997path} & Delay, Power, Area  \\
    			 & Strength reduction \cite{cooper2001operator}& Power, Area \\
    			 & Loop fusion \cite{darte1999complexity} & Power, Area \\
                 & Datapath pipelining \cite{teifel2004highly} & Delay \\
        \midrule
    Mux			
                 & Mux reduction \cite{chen2004register, wang2023optimization} & Delay, Power, Area \\
                 & Mux tree decomposition \cite{pivstekareduction} & Delay, Power, Area  \\
                & Mux tree restructuring \cite{wang2023optimization} & Delay, Power, Area  \\
    \midrule
    FSM          & State minimization \cite{kam2013synthesis} & Delay, Power, Area \\ 
                 & State assignment \cite{villa2012synthesis}  & Delay, Power, Area\\ 
              & State decomposition \cite{shelar1999decomposition}  & Delay, Power, Area\\ 
    \midrule
    Memory        & Memory sharing \cite{laforest2010efficient, ma2020hypervisor}& Power, Area \\ 
                  & Memory folding & Power, Area\\
                  & Memory banking \cite{zhou2017new,lai2019remap+}& Delay\\
                & Memory pipelining \cite{park2001synthesis}& Delay\\
    \bottomrule
    \end{tabular}
    \label{table:examples}
        }
    }
\end{table}
We provide analysis of Verilog code optimization case by case.

\newpage
\minisection{Resource sharing}
resource sharing is a powerful technique to optimize hardware designs by minimizing resource usage. By carefully managing when and how different operations use the shared resource, designers can achieve significant savings in terms of area, power, and complexity. This technique is particularly valuable in applications where operations can be serialized without impacting overall performance.

\minisection{Optimization instruction} 
Implementing resource sharing effectively involves several strategies and considerations:

\begin{itemize}
\item $\textit{Functional Sharing}$: Identifying opportunities where multiple operations can use the same hardware component. For example, an adder used in one part of a design might also be used in another part, provided the usage does not overlap in time.

\item $\textit{Multiplexing}$: Utilizing multiplexers to dynamically switch the connection of a shared resource to various parts of the circuit based on the operational phase or the control logic. This allows different parts of the design to use the same resource at different times.

\item $\textit{Controlled Resource Allocation}$: Developing a schedule or control logic that manages the time-sharing aspects of resources to avoid conflicts and ensure that data integrity is maintained throughout the operation.

\item $\textit{High-Level Synthesis }$: Using advanced synthesis tools that can automatically analyze code at a higher abstraction level (like C/C++) and determine the best ways to share resources when translating it into RTL. These tools often employ sophisticated algorithms to optimize resource usage.

\item $\textit{Design Space Exploration}$: Evaluating different resource sharing configurations to find the optimal balance between resource utilization and performance, considering factors like latency and throughput.
\end{itemize}

\minisection{Example} 

Suppose we have a design that requires adding two different sets of numbers at different times. Instead of using two separate adders, we can use a single adder and share it between the two operations.

\begin{figure}[h!]
\begin{minipage}{0.45\textwidth}
\lstinputlisting[caption=Without resource sharing, label={propagation}]{figs/appendix_example/without_resource_sharing.v}
\end{minipage}%
\hfill
\begin{minipage}{0.45\textwidth}
\lstinputlisting[caption=With resource sharing, label={propagation}]{figs/appendix_example/with_resource_sharing.v}
\end{minipage}%
\end{figure}
\newpage

\minisection{Subexpression elimination}
Subexpression elimination is an optimization technique used to identify and reuse common subexpressions within a hardware description. This reduces redundant computations, leading to more efficient hardware designs in terms of both resource usage and performance. By sharing the result of a common subexpression across multiple instances where it is used, designers can reduce the overall complexity of the hardware implementation.

\minisection{Optimization instruction}
Subexpression elimination typically involves the following steps:

\begin{itemize}
\item $\textit{Expression Identification}$: The compiler scans the code to identify expressions, especially those within loops or frequently called functions, which can benefit from optimization.

\item $\textit{Common Subexpression Detection}$: It looks for instances where the same expression appears more than once with the same input values and no intervening modifications that might alter the output.

\item $\textit{Expression Evaluation and Storage}$: The first instance of a common subexpression is evaluated, and the result is stored in a temporary variable.

\item $\textit{Replacement of Redundant Expressions}$: Subsequent instances of the same expression are replaced with the temporary variable, eliminating the need for re-evaluation.
\end{itemize}

\minisection{Example} 
\begin{figure}[h!]
\begin{minipage}{0.45\textwidth}
\lstinputlisting[caption=Without subexpression elimination, label={propagation}]{figs/appendix_example/without_subexpression_elimination.v}
\end{minipage}%
\hfill
\begin{minipage}{0.45\textwidth}
\lstinputlisting[caption=With subexpression elimination, label={propagation}]{figs/appendix_example/with_subexpression_elimination.v}
\end{minipage}%
\end{figure}
\newpage

Many applications in DSP, telecommunications, graphics, and control have computations that either involve a large number of multiplications of one variable with several constants or can easily be transformed to that form. This computation is referred to as a multiple constant multiplication (MCM) problem. 

 To solve the MCM problem, we first introduce multiplier blocks and the corresponding mathematical definition. A multiplier block implements multiplying a variable $x$ by a set of constants $t_{1},..., t_{n}$ in parallel. We define \textit{fundamentals} as a set of constants in a multiplier block.  We define an $\mathcal{A}$-operation as an operation on fundamentals. 
\begin{mydefinition}[General $\mathcal{A}$-operation]
Let $l_{1},l_{2} \geq 0$ be integers (left shifts),
$r \geq 0$ be an integer (right shift), and let $s \in \{0, 1\}$ (sign). An $\mathcal{A}$-operation is an
operation with two integer inputs $u$, $v$ (fundamentals) and one output fundamental,
defined as
\begin{equation}
\begin{split}
 \mathcal{A}_{p}(u,v) &= |(u<<l_{1}) + (-1)^{s}(v<<l_{2})|>>r\\
 & = \|2^{l_{1}}u +(-1)^{s}2^{l_{2}}v\|
 \end{split}
\end{equation}
where $<<$ and $>>$ are left shift and right shift, and $p=(l_{1}, l_{1}, r, s)$ is the $\mathcal{A}$-configuration of  $\mathcal{A}_{p}$
\end{mydefinition}

Now we formally introduce MCM problem as follows
\begin{mydefinition}[MCM problem]
Given a set of positive target constants $T=\{t_{0}, t_{1}, \cdot, t_{m}\} \in \mathbb{N}$. Find
the minimal set $R={r_{0}, r_{1}, \cdot, r_{m}}$ where $T \subset R$ such that $r_{0} =1$, and for all $r_{k}$ with $1\leq k \leq m$ there exist $r_{i}$, $r_{j}$ with $0\leq i$, $j<k$ and $\mathcal{A}$-configuration $p_{k}$ such that
\begin{equation}
r_{k} = \mathcal{A}_{p_{k}}(r_{i},r_{j})
\end{equation}
where $<<$ and $>>$ are left shift and right shift, and $p=(l_{1}, l_{1}, r, s)$ is the $\mathcal{A}$-configuration of  $\mathcal{A}_{p}$
\end{mydefinition}

The MCM problem is NP-complete. It can be solved by Algorithm 1.
\begin{algorithm}
\caption{Multiple Constant Multiplication (MCM) Optimization}
\begin{algorithmic}[1]
\State \textbf{Input:} Set of constants $\{C_1, C_2, \ldots, C_n\}$
\State \textbf{Output:} Optimized Verilog code with minimized multiplications

\Function{FindSubexpressions}{$C$}
    \State Initialize an empty dictionary $subexpressions$
    \For{each constant $C_i$ in $C$}
        \State $binary\_repr \gets \text{binary representation of } C_i$
        \State Initialize an empty list $shifts$
        \For{each bit $bit$ in $binary\_repr$ with index $i$}
            \If{$bit == 1$}
                \State $shifts.append(1 << i)$
            \EndIf
        \EndFor
        \State $subexpressions[C_i] \gets shifts$
    \EndFor
    \State \Return $subexpressions$
\EndFunction

\Function{OptimizeGraph}{$subexpressions$}
    \State Initialize an empty dictionary $graph$
    \For{each $constant$ and $shifts$ in $subexpressions$}
        \For{each $shift$ in $shifts$}
            \If{$shift \notin graph$}
                \State $graph[shift] \gets 0$
            \EndIf
            \State $graph[shift] \gets graph[shift] + 1$
        \EndFor
    \EndFor
    \State \Return $graph$
\EndFunction

\Function{GenerateVerilog}{$graph$}
    \State Initialize an empty list $verilog\_code$
    \For{each $shift$ and $count$ in $graph$}
        \State $verilog\_code.append("assign x\_shift = x << (\text{\texttt{bit\_length}}(shift) - 1);")$
    \EndFor
    \State \Return $verilog\_code$
\EndFunction

\State $constants \gets \{3, 5, 9\}$
\State $subexpressions \gets$ \Call{FindSubexpressions}{$constants$}
\State $optimized\_graph \gets$ \Call{OptimizeGraph}{$subexpressions$}
\State $verilog\_code \gets$ \Call{GenerateVerilog}{$optimized\_graph$}

\For{each $line$ in $verilog\_code$}
    \State Print $line$
\EndFor

\end{algorithmic}
\end{algorithm}

\minisection{Example} 
\begin{figure}[h!]
\begin{minipage}{0.45\textwidth}
\lstinputlisting[caption=Without mcm subexpression elimination, label={propagation}]{figs/appendix_example/without_mcm_subexpression_elimination.v}
\end{minipage}%
\hfill
\begin{minipage}{0.45\textwidth}
\lstinputlisting[caption=With mcm subexpression elimination, label={propagation}]{figs/appendix_example/with_mcm_subexpression_elimination.v}
\end{minipage}%
\end{figure}

\newpage
\minisection{Constant propagation}
Constant Propagation is one of the local code optimization techniques in Compiler Design. It can be defined as the process of replacing the constant value of variables in the expression. Constants assigned to a variable can be propagated through the flow graph and can be replaced when the variable is used. 

Constant propagation is a well-known global flow analysis problem. The goal of constant propagation is to discover values that are constant on all possible executions of a program and to propagate these constant values as far forward through the program as possible. Expressions whose operands are all constants can be evaluated at compile time and the results propagated further.

\begin{mydefinition}[Control flow graph]
A control flow graph (CFG) is composed of 
\begin{itemize}
\item $\text{Variables } v = x,y,....$ 
\item $\text{Constants } c = \mathbb{Z},\mathbb{N},....$ 
\item $\text{Expressions } e = v \leftarrow e , e_{1} + e_{2} , e_{1} - e_{2},....$ 
\end{itemize}
\end{mydefinition}

\begin{mydefinition}[Program]
A program is defined as a graph $(V,E,I)$ with 
\begin{itemize}
\item $V$ is a set of expressions in a control flow graph. 
\item $E\subset V \times V$ represents directed edges between expressions in $V$. $E = (e_{1}, e_{2})$ denotes the control flow from $e_{1}$ to $e_{2}$. $\text{succ}(e)=\{e'|(e, e')\in E\}$ denotes the immediate successors of a expression $e\in V$.
\item $I \subset V$ is a collection of entry points to the program.
\end{itemize}
\end{mydefinition}

Kildall’s algorithm is often used to solve constant propagation. It maintains a worklist $L \in \mathcal{P}((V \times P))$ of nodes to visit, and repeatedly propagates information through the program graph. If $(e, p) \in L$,
then expression $e$ has new information $p$ flowing into it from a predecessor
expression. We define two operations on worklist $L$
\begin{itemize}
\item $\text{pop}$: $L \rightarrow (V \times P)$ remove and return an arbitrary element of $L$.
\item $\cup$: an operation $L \times L \rightarrow L$ combines two worklist and remove duplicates.
\item $\wedge$: an operation $P \times P \rightarrow P$ such that the strict partial order $ p_{1}<p_{2} \equiv p_{1}\wedge p_{2} = p_{1}\wedge p_{1} \neq p_{2}$  
\end{itemize}
 \begin{algorithm}[h]
\begin{algorithmic}[1]
\Statex $\textbf{Input}:\text{A worklist }\boldsymbol{L}$;
\Statex $\textbf{Output}:\text{A updated worklist }\boldsymbol{L}$;

\State $L\leftarrow \{(I, \eta(i)|i \in I)\}$;  
\While {$L \neq \emptyset$}  
\State $(e, p_{i}) \leftarrow \text{pop}(L)$; 
\State $p_{e} \leftarrow \sum(e)$; 
\State $p_{e}^{+} \leftarrow p_{e} \ p_{i}$; 
\If $p_{e}^{+} \neq p_{e}$; 
\State $\sum(e) \leftarrow p_{e}^{+}$; 
\State $L \leftarrow L \cup \{ 
  (e',f(e, p_{e}^{+})) |e' \in \text{succ}(e)\} _{e}^{+}$; 
\EndIf
\EndWhile
\State $\textbf{return }L$;
\Statex $\}$
\caption{Kildall's algorithm}
\end{algorithmic}
\end{algorithm}

\minisection{Optimization instruction}
\begin{itemize}
\item $\textit{Identification of Constants}$: The first step involves scanning the program to identify constants—values that are known at compile time. Constants can be literal numbers, strings, or boolean values explicitly written in the code, or they can result from constant expressions that are computable during the compilation.

\item $\textit{Forward Propagation}$: Once constants are identified, the compiler propagates these values forward, replacing references to the constants with their actual values wherever possible. For instance, if a variable x is assigned the constant value 5, all subsequent uses of x within its scope can be replaced by the number 5, as long as x is not reassigned to a different value.

\item $\textit{Evaluation of Expressions}$: During propagation, the compiler also evaluates expressions that are fully determined by constants. For example, an expression like x + 10 where x is known to be 5 would be replaced by 15. This step effectively reduces the number of calculations needed at runtime.

\item $\textit{Code Simplification}$: This constant insertion can lead to further simplifications. For example, conditions in if-statements that evaluate to true or false can be resolved at compile time, potentially allowing whole blocks of code to be removed or replaced.
\end{itemize}

\minisection{Example} 
\begin{figure}[h!]
\begin{minipage}{0.45\textwidth}
\lstinputlisting[caption=Without constant propagation, label={propagation}]{figs/appendix_example/without_constant_propagation.v}
\end{minipage}%
\hfill
\begin{minipage}{0.45\textwidth}
\lstinputlisting[caption=With constant propagation, label={propagation}]{figs/appendix_example/with_constant_propagation.v}
\end{minipage}%
\end{figure}

\newpage
\minisection{Dead code elimination}
Dead code elimination is an optimization technique used in Verilog (as well as in other programming and hardware description languages) to remove parts of the code that do not affect the functionality of the design. Dead code typically includes variables, assignments, and operations that are never used or do not contribute to the output of the circuit. Eliminating dead code improves readability, reduces resource usage, and can enhance performance by simplifying the synthesized hardware.

The primary objectives of dead code elimination in RTL design are to reduce area, improve performance, and decrease power consumption. Specifically, by removing unused or unnecessary logic elements, the total area consumed by the circuit on the silicon can be significantly reduced. This is particularly important in cost-sensitive or space-constrained applications. Meanwhile, eliminating dead code can reduce the complexity of the circuit, potentially lowering propagation delays and improving the clock frequency. Moreover, less logic means lower power consumption, which is crucial for battery-operated devices and for reducing overall energy costs in large-scale deployments. Last, with less code to verify, the process of checking the design for errors becomes simpler and less prone to mistakes.

\begin{mydefinition}[DefUseChain]
A DefUseChain is a connection from a definition site for a variable to
a use site for that variable. This connection must be reachable along
the Program Flow Graph without passing through another definition site for that variable. Use sites are normally operands of expressions.
\end{mydefinition}

\begin{mydefinition}[DefJoinEdge and DefUseEdge]
We add new nodes called join nodes to the DefUseChain graph: One node is added for each use site. We divide
the DefUseChains into two parts: the first part, the DefJoinEdge, starts
at the definition site and terminates at a join node. The second part, the
JoinUseEdge, starts at the join node and terminates at the use site.
\end{mydefinition}

The dead code elimination algorithm is shown in Algorithm 4. This algorithm uses two worklists. The fit, FlowWorkList, is a worklist
of Program Flow Graph edges and the second, DefWorkList, is a worklist of DefJoinEdges.

\begin{algorithm}[h]
\caption{Dead Code Elimination Algorithm}
\begin{algorithmic}[1]
\Statex \textbf{Input:} A worklist \( \boldsymbol{L} \)
\Statex \textbf{Output:} An updated worklist \( \boldsymbol{L} \)

\Function{ConditionalDef}{}
    \State Initialize the edge entering the Start Node of the program in the FlowWorkList.
    \State Initialize LevelCells and ValueCells for the DefUseChain Graph.
    \State Initialize DefWorkList to empty.
    \State Set ExecutableFlag to false for all nodes, enabling expression evaluation.
    \State Halt execution when both worklists are empty; otherwise, process items from any worklist.
    \If{item is a Program Flow Graph edge from the FlowWorkList}
        \State Set ExecutableFlag to true.
        \If{ExecutableFlag was false}
            \State Evaluate the expression according to "Expression Rules."
            \If{result is not top}
                \State \Call{VisitExpression}{}
            \EndIf
        \EndIf
    \EndIf
    \If{item is a DefJoinEdge from the DefWorkList}
        \State Combine source value with value at the join node using "Meet Rules."
        \If{lattice value is lowered}
            \State Propagate new value to the expression.
            \If{ExecutableFlag is true}
                \State Evaluate the expression.
            \EndIf
        \EndIf
    \EndIf
\EndFunction

\Function{VisitExpression}{}
    \If{expression is part of an assignment node}
        \State Add all DefJoinEdges starting at the definition to the DefWorkList.
    \EndIf
    \If{expression controls a conditional branch}
        \State Add necessary flow graph edges to the FlowWorkList based on the branch outcome.
        \If{LevelCell has value bottom}
            \State Add both exit edges to the FlowWorkList.
        \Else
            \State Add the flow graph edge executed as a result of the branch to the FlowWorkList.
        \EndIf
    \EndIf
\EndFunction
\end{algorithmic}
\end{algorithm}

\minisection{Optimization instruction}
Dead code elimination in RTL involves several key steps:
\begin{itemize}
\item $\textit{Code Analysis}$: The RTL code is analyzed to identify any instances of unused or redundant logic. This includes unused variables, registers that are written but never read, and logic operations whose outputs do not influence observable outputs or the state of the system.

\item $\textit{Dependency Graph Construction}$: A dependency graph of the code is constructed, mapping out how different parts of the logic depend on each other. This helps in understanding the impact of removing a certain piece of code.

\item $\textit{Elimination of Redundant Logic}$: Using the dependency graph, logic that does not affect the final outputs or system state can be systematically removed. This step must be done carefully to ensure that no necessary functionality is lost.

\item $\textit{Optimization Passes}$: After the initial removal of dead code, further optimization passes may be necessary to refine the design and ensure that no new dead code has been introduced by the changes.

\item $\textit{Verification and Testing}$: Once the dead code has been eliminated, the modified RTL code must be thoroughly tested and verified against the original specifications to ensure that its behavior has not been altered in unintended ways.
\end{itemize}

\minisection{Example} 

\clearpage
\newpage
\minisection{Strenth reduction}
Strength reduction in RTL (Register Transfer Level) optimization refers to a technique used in the synthesis and optimization of digital circuits, where computationally expensive operations are replaced with simpler, less resource-intensive ones. This method aims to improve the overall efficiency of the hardware design, particularly in terms of speed, area, and power consumption.

The main goals of strength reduction in the context of RTL design are improving timing, reducing area and lowering power consumption. Specifically, by replacing slower operations with faster ones, the overall clock speed of the circuit can be improved. Meanwhile, simpler operations typically require fewer logic gates, which can reduce the silicon area needed for the circuit. Moreover, less complex operations generally consume less power, which is crucial for battery-operated devices and for reducing heat generation in high-performance systems.

\minisection{Optimization instruction}
Strength reduction often involves identifying opportunities to replace certain types of operations with others that have lower "strength" in terms of computational complexity and resource usage. Here are some common substitutions:
\begin{itemize}
\item $\textit{Multiplication by a Power of Two}$:
Instead of using a multiplier, you can use a shift operation.\\

\minisection{Example} 
\begin{figure}[h!]
\begin{minipage}{0.45\textwidth}
\lstinputlisting[caption=Without strength reduction, label={propagation}]{figs/appendix_example/multiply_by_4.v}
\end{minipage}%
\hfill
\begin{minipage}{0.45\textwidth}
\lstinputlisting[caption=With strength reduction, label={propagation}]{figs/appendix_example/multiply_by_4_opt.v}
\end{minipage}%
\end{figure}

\item $\textit{Division by a Power of Two}$:
Instead of using a divider, you can use a shift operation.\\
\minisection{Example} 
\begin{figure}[h!]
\begin{minipage}{0.45\textwidth}
\lstinputlisting[caption=Without strength reduction, label={propagation}]{figs/appendix_example/divide_by_8.v}
\end{minipage}%
\hfill
\begin{minipage}{0.45\textwidth}
\lstinputlisting[caption=With strength reduction, label={propagation}]{figs/appendix_example/divide_by_8_opt.v}
\end{minipage}%
\end{figure}

\item $\textit{Multiplication by a Constant}$:
Sometimes multiplication by a constant can be reduced using addition and shifts.\\
\minisection{Example} 
\begin{figure}[h!]
\begin{minipage}{0.45\textwidth}
\lstinputlisting[caption=Without strength reduction, label={propagation}]{figs/appendix_example/multiply_by_10.v}
\end{minipage}%
\hfill
\begin{minipage}{0.45\textwidth}
\lstinputlisting[caption=With strength reduction, label={propagation}]{figs/appendix_example/multiply_by_10_opt.v}
\end{minipage}%
\end{figure}

\newpage
\item $\textit{Boolean Algebra Simplifications}$:
Applying Boolean algebra to simplify expressions.\\
\minisection{Example} 
\begin{figure}[h!]
\begin{minipage}{0.45\textwidth}
\lstinputlisting[caption=Without strength reduction, label={propagation}]{figs/appendix_example/complex_boolean.v}
\end{minipage}%
\hfill
\begin{minipage}{0.45\textwidth}
\lstinputlisting[caption=With strength reduction, label={propagation}]{figs/appendix_example/complex_boolean_opt.v}
\end{minipage}%
\end{figure}

\item $\textit{Combining Operations}$:
Combining multiple operations to reduce the number of intermediate steps.\\
\minisection{Example} 
\begin{figure}[h!]
\begin{minipage}{0.45\textwidth}
\lstinputlisting[caption=Without strength reduction, label={propagation}]{figs/appendix_example/combined_operation.v}
\end{minipage}%
\hfill
\begin{minipage}{0.45\textwidth}
\lstinputlisting[caption=With strength reduction, label={propagation}]{figs/appendix_example/combined_operation_opt.v}
\end{minipage}%
\end{figure}
\end{itemize}

\clearpage
\newpage
\minisection{Mux reduction}
Mux reduction in RTL (Register Transfer Level) design is an optimization technique aimed at reducing the number and complexity of multiplexers (muxes) in digital circuits. Multiplexers are critical components in digital designs, used to select one of many input signals based on a control signal. By reducing the number and size of muxes, the overall hardware efficiency, performance, and cost of the design can be optimized.

Mux reduction primarily focuses on area optimization, power efficiency, and performance improvement. Specifically, fewer or smaller multiplexers lead to a reduction in the silicon area required, which directly impacts the cost and scalability of the hardware. Meanwhile, smaller, fewer, or more efficient mux structures consume less power, which is crucial in low-power applications and reduces overall energy consumption. In addition, reducing the complexity and number of muxes can decrease signal propagation delays, improving the circuit's overall performance.

\minisection{Optimization instruction}

Several strategies can be employed to reduce the use of muxes in RTL design:
\begin{itemize}
\item $\textit{Sharing Muxes}$: Identifying opportunities where multiple logical functions can share the same mux. This often involves clever circuit design or leveraging specific characteristics of the logic being implemented.

\item $\textit{Logic Simplification}$: Simplifying the Boolean expressions and logic design to minimize the conditions under which multiplexing is needed. Techniques like Boolean algebra, Karnaugh maps, or software tools for logic minimization can be helpful.

\item $\textit{Mux Consolidation}$: Combining several smaller muxes into a single, larger multiplexer when the control logic can be efficiently managed. This might involve reorganizing how data paths are controlled and might be beneficial when it simplifies the overall design.

\item $\textit{Optimal Control Signal Generation}$: Optimizing the generation of control signals for muxes can sometimes reduce the number of mux inputs required or the complexity of the control logic itself.

% \item $\textit{Advanced Synthesis Optimizations}$: Utilizing synthesis tools that can automatically identify and implement mux reduction opportunities based on the target technology (e.g., ASIC, FPGA). These tools analyze the RTL description and apply hardware-specific optimizations.
\end{itemize}

\minisection{Example} 
\begin{figure}[h!]
\begin{minipage}{0.45\textwidth}
\lstinputlisting[caption=Without mux reduction, label={propagation}]{figs/appendix_example/with_mux_reduction.v}
\end{minipage}%
\hfill
\begin{minipage}{0.45\textwidth}
\lstinputlisting[caption=With mux reduction, label={propagation}]{figs/appendix_example/without_mux_reduction.v}
\end{minipage}%
\end{figure}

\clearpage
\newpage
\minisection{Mux restructuring}
Multiplexer restructuring is a technique used in digital circuit design, particularly in the optimization of logic circuits. This process involves transforming portions of a digital circuit to utilize multiplexers (muxes) effectively, potentially reducing the complexity, area, and power consumption of the circuit. 

The key concepts of mux restructuring include reorganizing select logic, which involves altering the arrangement of select lines to simplify and reduce the complexity of the circuit. Another concept is combining multiplexers, which entails merging multiple small multiplexers into a single, larger multiplexer. Additionally, breaking down large multiplexers refers to dividing a large multiplexer into smaller, more manageable parts to simplify the design.

Mux restructuring offers several benefits. Firstly, it reduces logic depth by integrating multiple layers of multiplexers into a single conditional statement, thereby decreasing the number of gate delays and enhancing performance. Secondly, it simplifies the design, making it more straightforward and easier to maintain due to fewer intermediate signals and reduced levels of logic. Lastly, it optimizes resource usage, requiring fewer logic elements, which leads to lower resource consumption in the synthesized hardware and can also result in reduced power consumption.

\begin{mydefinition}[Mux]
a multiplexer (or mux), also known as a data selector, is a device that selects between several analog or digital input signals and forwards the selected input to a single output line. The selection is directed by a separate set of digital inputs known as select lines. A multiplexer of 
 $2^{n}$ inputs have $n$ select lines, which are used to select which input line to send to the output.
\end{mydefinition}

\minisection{Optimization instruction}
Multiplexer restructuring involves analyzing a given digital logic circuit to identify opportunities where multiple logic gates or complex logic expressions can be replaced with simpler mux-based structures. Here’s how it generally works:
\begin{itemize}
\item $\textit{Circuit Analysis}$: The original logic circuit is analyzed to identify potential optimizations. This includes determining the dependencies and relationships between different logic outputs and inputs.

\item $\textit{Identification of Multiplexer Opportunities}$: Specific areas of the circuit where the logic functions can be effectively represented as selections between inputs based on control signals are identified. This often involves boolean algebra simplification and dependency analysis.

\item $\textit{Design of Multiplexer-Based Logic}$: The identified functions are redesigned to use multiplexers. This involves choosing the appropriate size and type of multiplexer and designing the control logic that determines which inputs are selected under different conditions.

\item $\textit{Implementation and Testing}$: The new circuit design is implemented, either in hardware or simulation, to verify that it meets all the functional requirements. Performance metrics such as timing, power consumption, and resource utilization are evaluated.

\item $\textit{Optimization}$: Based on the testing results, further adjustments might be made to the multiplexer configurations to enhance performance or reduce resource usage.
\end{itemize}

\minisection{Example} 
\begin{figure}[h!]
\begin{minipage}{0.45\textwidth}
\lstinputlisting[caption=Without mux restructuring, label={propagation}]{figs/appendix_example/with_mux_restructuring.v}
\end{minipage}%
\hfill
\begin{minipage}{0.45\textwidth}
\lstinputlisting[caption=With mux restructuring, label={propagation}]{figs/appendix_example/without_mux_restructuring.v}
\end{minipage}%
\end{figure}

\clearpage
\newpage
\minisection{State reduction}
 state reduction is a process used in digital design to minimize the number of states in a finite state machine (FSM) without altering its functionality. 
The steps for state reduction involve several key actions. First, identify equivalent states by determining pairs that exhibit identical behavior in terms of outputs and transitions. Next, merge these equivalent states into a single state. Following this, update the state transition logic to reflect the changes made by the merging process. Finally, optimize the state encoding by reassigning state encodings if necessary to enhance the overall design.

\begin{mydefinition}[Finite State Machine]
A Finite State Machine is defined by \((\Sigma, S, s_0, \delta, F, O)\), where

    \(\Sigma\) is the input alphabet, a finite, non-empty set of symbols.\\
    \(S\) is a finite, non-empty set of states.\\
    \(s_0\) is the initial state, an element of \(S\).\\
    \(\delta\) is the state-transition function: \(\delta : S \times \Sigma \to S\).\\
   \(F\) is the set of final states, a (possibly empty) subset of \(S\).\\
    \(O\) is the set of outputs.\\

\end{mydefinition}

Hopcroft's algorithm, as shown in Algorithm 5, is often used for state reduction.
\begin{algorithm}[H]
\caption{Hopcroft's Algorithm}
\begin{algorithmic}[1]
\Statex $\textbf{input: }$ A DFA $(Q, \Sigma, \delta, q_0, F)$
\Statex $\textbf{output: }$ The minimized DFA

\State $P \leftarrow \{F, Q \setminus F\}$ \Comment{Partition the states into final and non-final states}
\State $W \leftarrow \{F\}$ \Comment{Initialize the worklist with the set of final states}

\While{$W \neq \emptyset$}
    \State Remove a set $A$ from $W$
    \For{ $c \in \Sigma$ }
        \State Let $X \leftarrow \{ q \in Q \mid \delta(q, c) \in A \}$
        \For{ $Y \in P$ }
            \State Let $Y_1 \leftarrow Y \cap X$ 
            \State Let $Y_2 \leftarrow Y \setminus X$
            \If{ $Y_1 \neq \emptyset$ and $Y_2 \neq \emptyset$ }
                \State Replace $Y$ in $P$ by $Y_1$ and $Y_2$
                \If{ $Y \in W$ }
                    \State Replace $Y$ in $W$ by $Y_1$ and $Y_2$
                \Else
                    \If{ $|Y_1| \leq |Y_2|$ }
                        \State Add $Y_1$ to $W$
                    \Else
                        \State Add $Y_2$ to $W$
                    \EndIf
                \EndIf
            \EndIf
        \EndFor
    \EndFor
\EndWhile
\Statex $\textbf{return }P$ \Comment{The partition $P$ now describes the sets of equivalent states}
\end{algorithmic}
\end{algorithm}

The benefits of state reduction include a simplified design, as having fewer states makes the finite state machine (FSM) easier to understand, debug, and maintain. Additionally, improved performance is achieved through reduced logic complexity, which can result in faster operation due to fewer state transitions and simpler state encoding. Finally, resource optimization occurs because fewer states lead to reduced usage of flip-flops and combinational logic in the synthesized hardware, ultimately resulting in lower power consumption and cost.

\minisection{Optimization instruction}
The two primary methods for reducing states in an FSM are elimination of unreachable states and merging of equivalent states.
\begin{itemize}
 \item $\textit{Elimination of unreachable states}$: These are states that cannot be reached from the initial state under any input conditions. Since these states do not affect the FSM's operation, they can be removed entirely. 
 
  \item $\textit{Merging of equivalent states}$: this involves identifying states that are indistinguishable in terms of their response to a given set of inputs and their subsequent behavior. Two states are considered equivalent if, for every possible input, they
transit to the same next state or to equivalent states. Meanwhile, they
produce the same output (in the case of a Moore machine) or have identical output behavior for corresponding transitions (in the case of a Mealy machine).
\end{itemize}

\minisection{Example} 
\begin{figure}[h!]
\begin{minipage}{0.45\textwidth}
\lstinputlisting[caption=Without state reduction, label={propagation}]{figs/appendix_example/without_state_reduction.v}
\end{minipage}%
\hfill
\begin{minipage}{0.45\textwidth}
\lstinputlisting[caption=With state reduction, label={propagation}]{figs/appendix_example/with_state_reduction.v}
\end{minipage}%
\end{figure}

\clearpage
\newpage
\minisection{State assignment}
Verilog state assignment refers to the process of assigning binary values to the states of a finite state machine (FSM) in digital design. Proper state assignment is crucial because it can impact the performance, complexity, and resource utilization of the FSM. There are several methods for state assignment, each with its own advantages and considerations.

Binary encoding involves assigning each state a unique binary number. This method is straightforward but not necessarily optimal for minimizing the complexity of the transition logic. One-hot encoding represents each state with a binary code where only one bit is '1', and all other bits are '0'. This approach often leads to simpler and faster transition circuits at the cost of using more memory or logic elements. Gray code encoding assigns states such that only one bit changes between successive states. This can minimize the risk of error in state transitions, particularly in asynchronous designs. Custom encoding involves using algorithms to determine an optimal encoding scheme based on the specific transition frequencies and patterns within the FSM. This approach can significantly reduce logic complexity but requires more sophisticated design tools or algorithms.

A state assignment algorithm is shown in Algorithm 6.
\begin{algorithm}
\caption{State Assignment for Finite State Machines}
\begin{algorithmic}[1]
\Statex \textbf{Input:} A set of states \( S \), A set of transitions \( T \) with each transition as a tuple \( (s_i, s_j) \)
\Statex \textbf{Output:} A mapping of each state to a unique binary code

\Procedure{AssignStates}{$S$, $T$}
    \State $graph \gets$ \Call{BuildGraph}{$S$, $T$}
    \State $transition\_frequency \gets$ \Call{CalculateFrequencies}{$T$}
    \State $sorted\_transitions \gets$ \Call{SortByFrequency}{$transition\_frequency$}
    \State $code\_assignment \gets$ empty dictionary
    \State $code\_counter \gets 0$
    
    \For{each $(s_i, s_j)$ in $sorted\_transitions$}
        \If{$s_i \notin code\_assignment$ and $s_j \notin code\_assignment$}
            \State $code\_assignment[s_i] \gets \text{format}(code\_counter, 'b')$
            \State $code\_assignment[s_j] \gets \text{format}(code\_counter + 1, 'b')$
            \State $code\_counter \gets code\_counter + 2$
        \ElsIf{$s_i \in code\_assignment$ and $s_j \notin code\_assignment$}
            \State $code\_assignment[s_j] \gets \text{format}(code\_counter, 'b')$
            \State $code\_counter \gets code\_counter + 1$
        \ElsIf{$s_j \in code\_assignment$ and $s_i \notin code\_assignment$}
            \State $code\_assignment[s_i] \gets \text{format}(code\_counter, 'b')$
            \State $code\_counter \gets code\_counter + 1$
        \EndIf
    \EndFor

    \For{each $s$ in $S$}
        \If{$s \notin code\_assignment$}
            \State $code\_assignment[s] \gets \text{format}(code\_counter, 'b')$
            \State $code\_counter \gets code\_counter + 1$
        \EndIf
    \EndFor

    \State \Return $code\_assignment$
\EndProcedure
\end{algorithmic}
\end{algorithm}

\minisection{Optimization instruction}
Advanced methods use algorithms and heuristics to find an optimal or near-optimal assignment of binary codes to states:

\begin{itemize}
\item $\textit{Sequential Techniques}$: These methods consider one state at a time, assigning codes in a way that builds on the previous assignments to optimize the overall design.

\item $\textit{Combinatorial Optimization}$: Techniques such as genetic algorithms, simulated annealing, or integer linear programming can be used to explore a broader set of potential state assignments and find an efficient configuration.
\end{itemize}

\minisection{Example} 
\begin{figure}[h!]
\begin{minipage}{0.45\textwidth}
\lstinputlisting[caption=Without state assignment, label={propagation}]{figs/appendix_example/without_state_assignment.v}
\end{minipage}%
\hfill
\begin{minipage}{0.45\textwidth}
\lstinputlisting[caption=With state assignment, label={propagation}]{figs/appendix_example/with_state_assignment.v}
\end{minipage}%
\end{figure}

\clearpage
\newpage
\minisection{Memory sharing}
Memory sharing in digital design and computer architecture refers to the practice of allowing multiple components, processes, or threads to access and use the same physical memory resources. This technique is employed to optimize resource utilization, improve performance, and facilitate communication between different parts of a system. Memory sharing can be implemented in various ways, depending on the specific requirements and architecture of the system.

There are several benefits of resource sharing. Resource optimization is achieved by sharing memory, which reduces the total amount of memory required and leads to more efficient use of hardware resources. Improved performance is another benefit, as shared memory allows for faster data exchange between processes compared to other communication methods like message passing or file I/O. Additionally, communication is simplified because processes can communicate more easily and efficiently by reading from and writing to shared memory segments.

\minisection{Optimization instruction}
Several strategies can be employed to implement memory sharing in RTL design:

\begin{itemize}
\item$\textit{Resource Allocation and Scheduling}$: Analyze the usage patterns of different memory elements to identify opportunities where multiple processes or data paths can use the same memory resource at different times or under different conditions.

\item$\textit{Banked Memory}$: Implement a memory architecture where multiple smaller memory banks are used instead of a single large block. Each bank can be independently accessed, allowing multiple units to share the memory system effectively without interference.

\item$\textit{Multiplexing Memory Access}$: Use multiplexers to control access to memory elements so that they can be shared among multiple data paths or processing units. The mux selects which unit gets access to the memory at any given cycle based on control logic that ensures data integrity and correct operation.

\item$\textit{Dynamic Memory Management}$: Employ a dynamic management strategy that allocates and deallocates memory in real-time based on the current needs of the system, much like memory management in software systems but implemented at the hardware level.

\item$\textit{Overlaying}$: : Store different data items in the same memory location at different times, based on a careful analysis of the lifetimes of these data items. This is particularly useful in FPGA implementations where reconfigurability allows for flexible use of memory resources.
\end{itemize}

\minisection{Example} 
\begin{figure}[h!]
\begin{minipage}{0.45\textwidth}
\lstinputlisting[caption=Without memory sharing, label={propagation}]{figs/appendix_example/without_memory_sharing.v}
\end{minipage}%
\hfill
\begin{minipage}{0.45\textwidth}
\lstinputlisting[caption=With memory sharing, label={propagation}]{figs/appendix_example/with_memory_sharing.v}
\end{minipage}%
\end{figure}
\clearpage
\newpage
\minisection{Memory folding}
In digital design, especially when working with FPGA or ASIC implementations, memory resources are often limited. Designers aim to make efficient use of these resources to meet design constraints such as area, power consumption, and performance.

Memory folding is a method where multiple smaller memory blocks (which could be separate arrays or different segments of data) are folded into a single larger memory block. This is done to optimize the usage of memory resources, reduce area, and sometimes improve access times.

The main objectives of memory folding in RTL design are to reduce area, power, and cost. Specifically, by folding memory, the silicon area dedicated to memory components can be substantially decreased, which is crucial for reducing manufacturing costs and enhancing the compactness of the design.
Meanwhile, smaller memory configurations consume less power, which is important for energy conservation and extending battery life in portable devices. Moreover, minimizing the amount of memory used in a design directly impacts the overall cost of the device, making it more economically viable, especially in high-volume production.

\minisection{Optimization instruction}
Memory folding typically involves several key strategies:
\begin{itemize}
\item $\textit{Time-Multiplexed Memory Access}$: This strategy utilizes the fact that certain memory elements are not needed at all times during the operation of a circuit. Memory resources can be shared across multiple functionalities by ensuring that their access times do not overlap.

\item $\textit{Variable Lifetime Analysis}$: By analyzing the lifetimes of various variables stored in memory, those that do not have overlapping lifetimes can share the same memory space. This requires a careful analysis of when variables are written to and read from memory throughout the program execution.

\item$\textit{Overlapping Data Storage}$: Similar to variable lifetime analysis, this involves storing data in a way that maximizes the use of available memory by overlapping data storage in the same memory locations at different times or under different operational modes.

\item$\textit{Memory Segmentation and Alignment}$: In some cases, memory can be segmented into smaller parts, and different data types or structures can be aligned in such a way that maximizes the usage efficiency of each segment.

\item$\textit{Dynamic Memory Reconfiguration}$: Particularly relevant in FPGA implementations and other reconfigurable computing platforms, dynamic memory reconfiguration allows the memory structure to be changed in real-time based on current operational needs, further enhancing memory usage efficiency.
\end{itemize}

\minisection{Example} 
\begin{figure}[h!]
\begin{minipage}{0.45\textwidth}
\lstinputlisting[caption=Without memory folding, label={propagation}]{figs/appendix_example/without_memory_folding.v}
\end{minipage}%
\hfill
\begin{minipage}{0.45\textwidth}
\lstinputlisting[caption=With memory folding, label={propagation}]{figs/appendix_example/with_memory_folding.v}
\end{minipage}%
\end{figure}
